# Supplementary material for: Translational diffusion coefficients of membrane protein aggregates in free and supported lipid membranes
Source: arXiv:2512.01090 ancillary file (2025-11-30)
Supplement: Supplementary file 1 [file AggDiff_SI.pdf]

# Supplementary Material

## Translational diffusion coefficients of membrane protein aggregates in free and supported lipid membranes

Yannick A. D. Omar \*

Department of Chemical Engineering, Massachusetts Institute of Technology, Cambridge, Massachusetts, 02139, USA

### Contents

|          |                                                                     |           |
|----------|---------------------------------------------------------------------|-----------|
| <b>1</b> | <b>On the positive definiteness of the mobility tensor</b>          | <b>1</b>  |
| 1.1      | Free-standing lipid membranes — $r_{ij} \ll \ell_{SD}$              | 2         |
| 1.2      | Free-standing lipid membranes — general $r_{ij}$                    | 5         |
| <b>2</b> | <b>Mobility tensor in the Evans–Sackmann theory</b>                 | <b>8</b>  |
| 2.1      | Stokeslet approximation                                             | 8         |
| 2.2      | Yamakawa’s method for a membrane near a wall                        | 10        |
| 2.3      | Stokeslet approximation based on original Evans–Sackmann derivation | 11        |
| 2.4      | Positive definiteness of the mobility tensor                        | 12        |
| <b>3</b> | <b>Derivation of the hydrodynamic radii</b>                         | <b>15</b> |
| 3.1      | Free-standing membrane                                              | 16        |
| 3.2      | Membrane near a wall                                                | 17        |
|          | <b>Supporting References</b>                                        | <b>18</b> |

## 1 On the positive definiteness of the mobility tensor

While the theory of Kirkwood and Riseman is formulated using a generic tensor representing hydrodynamic interactions [1], the original article uses a point-particle or Stokeslet approximation when applying the theory to linear polymers. Zwanzig and coworkers [2] later showed that the Stokeslet approximation can lead to singularities and negative diffusion coefficients for strong hydrodynamic couplings. Both effects are a direct result of the mobility tensor losing its positive definiteness. It is important to note, however, that Zwanzig and coworkers recognized that this is an effect that can only arise when  $r_{ij} \leq R^S < 2a$ , for the interparticle distances  $r_{ij}$ , some upper bound  $R^S$  and particle radii  $a$  [3]. A similar observation was also made in Ref. [4].

To alleviate this issue, the seminal work by Rotne and Prager related the loss of positive definiteness to the dissipation turning negative at small particle distances [5]. The authors then devised a method for constructing a positive-definite hydrodynamic coupling tensor by requiring dissipation to be positive. However, because the method does not consider overlapping particles, it still leads to a loss of positive definiteness for particle distances  $r_{ij} \leq R^{\text{RPY}} < 2a$ , for some bound  $R^{\text{RPY}}$  [3].

---

\*yadomar@mit.edu

Simultaneously, Yamakawa formulated an alternative method to incorporate finite-size corrections into the Kirkwood-Riseman theory by distributing the point force and velocity perturbation of the Stokeslet approximation over finite-size spheres and averaging appropriately [6]. This led to the same results as in the work of Rotne and Prager. Yamakawa further showed that the finite-size correction should be viewed as a first-order correction to the Stokeslet approximation. Therefore, the Rotne-Prager-Yamakawa tensor should not be viewed as a remedy to the loss of positive definiteness in the Stokeslet approximation<sup>1</sup>, but rather as a more accurate representation of hydrodynamic interactions at small particle distances.

### 1.1 Free-standing lipid membranes — $r_{ij} \ll \ell_{\text{SD}}$

In this section, we show that the mobility tensor obtained from the Stokeslet approximation in free-standing lipid membranes (Saffman-Delbrück limit) may also lose its positive definiteness for overlapping particles. However, we begin by discussing the approach by Sokolov and Diamant to derive a positive definite hydrodynamic interaction tensor for lipid membranes [7], which closely parallels the work by Rotne and Prager [5]. To this end, we consider the dissipation due to the in-plane force  $\mathbf{F}_i$  on particle  $i$  in a collection of  $N$  particles. By introducing the  $2N \times 1$  global force vector,  $\mathbf{F} = [\mathbf{F}_1, \dots, \mathbf{F}_N]$ , and the  $2N \times 2N$  mobility tensor  $\mathbf{T}^g$ , which maps forces on particle  $i$  to velocity perturbations at particle  $j$ , we can express the power imparted on the membrane as  $\mathbf{F} \cdot \mathbf{T}^g \mathbf{F}$ . This power has to be balanced by the dissipation in the membrane and bulk fluid arising from shear stresses, i.e.

$$\mathbf{F} \cdot \mathbf{T}^g \mathbf{F} = \frac{1}{2\zeta} \int_{\mathcal{S}} da \, \boldsymbol{\tau}^m : \boldsymbol{\tau}^m + \frac{1}{2\eta} \int_{\mathcal{B}} dv \, \boldsymbol{\tau}^b : \boldsymbol{\tau}^b, \quad (1)$$

where  $\mathcal{S}$  is the membrane domain excluding the location of the particles,  $\mathcal{B}$  is the bulk fluid domain,  $\zeta$  and  $\eta$  are the membrane and bulk viscosities, respectively, and the membrane and bulk shear stresses are given by

$$\boldsymbol{\tau}^m = \zeta \left( \nabla^s \mathbf{v} + (\nabla^s \mathbf{v})^T \right), \quad (2)$$

$$\boldsymbol{\tau}^b = \eta \left( \nabla \mathbf{u} + (\nabla \mathbf{u})^T \right), \quad (3)$$

in terms of the surface gradient  $\nabla^s$  and membrane and bulk velocities  $\mathbf{v}$  and  $\mathbf{u}$ , respectively. Next, we note  $\text{tr} \boldsymbol{\tau}^m = 0$  and that the membrane linear momentum balance can be written as [8, 9]

$$\text{div}_s \left( \underbrace{\lambda \mathbf{I}_s + \boldsymbol{\tau}^m}_{\boldsymbol{\sigma}^m} \right) + (\mathbf{t}^+ + \mathbf{t}^-) = \mathbf{0}, \quad (4)$$

where  $\text{div}_s$  is the surface divergence,  $\lambda$  is the membrane tension,  $\mathbf{I}_s$  is the two-dimensional unit tensor, and  $\mathbf{t}^\pm$  are the tractions acting on the membrane from the bulk domains above and below the membrane. Rewriting Eq. (1), we obtain

$$\mathbf{F} \cdot \mathbf{T}^g \mathbf{F} = \int_{\mathcal{S}} da \, \text{div}_s (\mathbf{v} \cdot \boldsymbol{\sigma}^m) + \int_{\mathcal{S}} da \, \mathbf{v} \cdot (\mathbf{t}^+ + \mathbf{t}^-) + \frac{1}{2\eta} \int_{\mathcal{B}} dv \, \boldsymbol{\tau}^b : \boldsymbol{\tau}^b. \quad (5)$$

---

<sup>1</sup>A correction to the Rotne-Prager-Yamakawa tensor for arbitrarily overlapping particles is derived in Ref. [3].

Here, the second integral is the negative of the power the membranes exerted on the bulk fluid such that the total dissipation reduces to

$$\mathbf{F} \cdot \mathbf{T}^g \mathbf{F} = \int_{\mathcal{S}} da \operatorname{div}_s(\mathbf{v} \cdot \boldsymbol{\sigma}^m) . \quad (6)$$

In Ref. [7], the authors use Eq. (6) as the starting point.

Decomposing the stress and velocities into per-particle contributions leads to

$$\boldsymbol{\sigma}^m(\mathbf{x}) = \sum_i \boldsymbol{\sigma}_i^m(\mathbf{x} - \mathbf{r}_i) , \quad (7)$$

$$\mathbf{v}(\mathbf{x}) = \sum_i \mathbf{v}_i(\mathbf{x} - \mathbf{r}_i) , \quad (8)$$

where  $\mathbf{r}_i$  is the location of particle  $i$ . Furthermore, following Refs. [5, 7], we extend the definition of the stresses  $\boldsymbol{\sigma}_i^m$  and velocities  $\mathbf{v}_i$  into the domains of all other particles  $j \neq i$ . Then, Eq. (6) can be written in terms of an approximate mobility tensor as

$$\mathbf{F} \cdot \bar{\mathbf{T}}^g \mathbf{F} = \sum_{i,j} \int_{\partial\mathcal{S}_j} ds \mathbf{v}_i(\mathbf{x}) \cdot \boldsymbol{\sigma}_j^m(\mathbf{x} + \mathbf{r}_i - \mathbf{r}_j) \mathbf{n}^j(\mathbf{x}) , \quad (9)$$

with  $\partial\mathcal{S}_j$  being the boundary of particle  $j$  with outward-pointing normal  $\mathbf{n}^j$ . Under the assumption of small interparticle distances,  $r_{ij} \ll \ell_{\text{SD}}$ , Sokolov and Diamant then find [7]

$$\bar{\mathbf{T}}^g = \begin{bmatrix} \mathbf{T}_{11}^{\text{SD}} & \dots & \mathbf{T}_{1N}^{\text{SD}} \\ \vdots & \ddots & \vdots \\ \mathbf{T}_{N1}^{\text{SD}} & \dots & \mathbf{T}_{NN}^{\text{SD}} \end{bmatrix} , \quad (10)$$

with

$$\mathbf{T}_{ii}^{\text{SD}} = \frac{1}{4\pi\zeta} \left( \ln\left(\frac{2\ell_{\text{SD}}}{a}\right) - \gamma \right) \mathbf{I}_s , \quad (11)$$

$$\mathbf{T}_{ij}^{\text{SD}} = \frac{1}{4\pi\zeta} \left[ \left( \ln\left(\frac{2\ell_{\text{SD}}}{r_{ij}}\right) - \gamma - \frac{1}{2} + \frac{a^2}{r_{ij}^2} \right) \mathbf{I}_s + \left( 1 - 2\frac{a^2}{r_{ij}^2} \right) \frac{\mathbf{r}_{ij} \otimes \mathbf{r}_{ij}}{r_{ij}^2} \right] , \quad (12)$$

where  $\gamma$  is the Euler–Mascheroni constant,  $\mathbf{I}_s$  is the in-plane identity tensor, and  $\mathbf{r}_{ij}$  is the interparticle distance vector with norm  $r_{ij}$ . We note here that the diagonal terms  $\mathbf{T}_{ii}^{\text{SD}}$  do not explicitly appear in Kirkwood-Riseman theory, described in the main text. However, the force balance of Kirkwood-Riseman theory can be rewritten as  $\bar{\mathbf{T}}^g \bar{\mathbf{F}} = \bar{\mathbf{w}}$  in terms of the global force vector  $\bar{\mathbf{F}} = [\mathbf{F}_1^T, \dots, \mathbf{F}_N^T]^T$  and velocity vector  $\bar{\mathbf{w}} = [\mathbf{w}^T, \dots, \mathbf{w}^T]^T$  (see main text for details), showing consistency with the approach described above.

To investigate the positive definiteness of  $\bar{\mathbf{T}}^g$ , we rewrite the left-hand side of Eq. (9) as

$$\mathbf{F} \cdot \bar{\mathbf{T}}^g \mathbf{F} = \sum_{i,j} \mathbf{F}^i \mathbf{T}_{ij}^{\text{SD}} \mathbf{F}^j , \quad (13)$$

and note that  $\mathbf{T}_{ij}^{\text{SD}}$  depends only on the location of particles  $i$  and  $j$ , independent of the locations of all other particles. This shows that positive definiteness of the pairwise mobility tensor  $\mathbf{T}_{ij}^{\text{SD}}$  is

a sufficient criterion for positive definiteness of  $\bar{\mathbf{T}}^g$ . Moreover, since we require positive definiteness for any collection of particles, including when  $N = 2$ , the pairwise condition is also necessary. To further simplify the following discussion, we rewrite Eqs. (11) and (12) in the generic format

$$\mathbf{T}_{ii}^{\text{SD}} = h\mathbf{I}_s , \quad (14)$$

$$\mathbf{T}_{ij}^{\text{SD}} = f(r_{ij})\mathbf{I}_s + g(r_{ij})\frac{\mathbf{r}_{ij} \otimes \mathbf{r}_{ij}}{r_{ij}^2} , \quad (15)$$

with

$$h = \frac{1}{4\pi\zeta} \left( \ln\left(\frac{2\ell_{\text{SD}}}{a}\right) - \gamma \right) , \quad (16)$$

$$f(r_{ij}) = \frac{1}{4\pi\zeta} \left( \ln\left(\frac{2\ell_{\text{SD}}}{r_{ij}}\right) - \gamma - \frac{1}{2} + \frac{a^2}{r_{ij}^2} \right) , \quad (17)$$

$$g(r_{ij}) = \frac{1}{4\pi\zeta} \left( 1 - 2\frac{a^2}{r_{ij}^2} \right) . \quad (18)$$

By setting  $r_{12} = r_{21} = r$ , the eigenvalues of  $\bar{\mathbf{T}}^g$  for the two-particle system are given by

$$\lambda_1 = h + f(r) , \quad (19)$$

$$\lambda_2 = h - f(r) , \quad (20)$$

$$\lambda_3 = h - f(r) - g(r) , \quad (21)$$

$$\lambda_4 = h + f(r) + g(r) . \quad (22)$$

The tensor  $\bar{\mathbf{T}}^g$  loses its positive definiteness when at least one of the eigenvalues is negative.

We begin by considering the Stokeslet approximation, obtained by setting  $a = 0$  in Eqs. (17) and (18). Then, each of the eigenvalues  $\lambda_i$  has one root, located, respectively, at

$$r_1^* = \frac{4\ell_{\text{SD}}^2}{a} e^{-2\gamma - \frac{1}{2}} \gg \ell_{\text{SD}} , \quad (23)$$

$$r_2^* = ae^{-\frac{1}{2}} \approx 0.61a < 2a , \quad (24)$$

$$r_3^* = ae^{\frac{1}{2}} \approx 1.65a < 2a , \quad (25)$$

$$r_4^* = \frac{4\ell_{\text{SD}}^2}{a} e^{-2\gamma + \frac{1}{2}} \gg \ell_{\text{SD}} . \quad (26)$$

Furthermore, we find  $\lambda_1(r < r_1^*) > 0$ ,  $\lambda_4(r < r_4^*) > 0$  and  $\lambda_2(r < r_2^*) < 0$ ,  $\lambda_3(r < r_3^*) < 0$ . Thus,  $\lambda_2$  and  $\lambda_3$  become negative for small particle distances while  $\lambda_1$  and  $\lambda_4$  become negative at large particle distances. The latter is an artifact of assuming  $r \ll \ell_{\text{SD}}$ , as will be discussed in the next section.

When we consider the finite-size corrections in Eqs. (17) and (18), we find the positive roots of

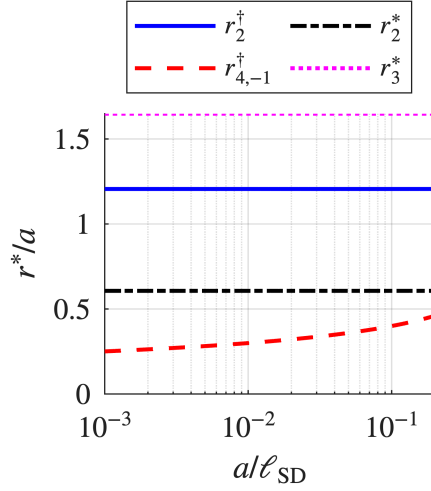

Figure 1: Roots associated with the loss of positive definiteness of the pairwise mobility tensor for the Stokeslet (\*) and Rotne–Prager–Yamakawa-type approximations (†).

the eigenvalues  $\lambda_1$ ,  $\lambda_2$  and  $\lambda_4$  as,

$$r_1^\dagger = a \sqrt{\frac{2}{W_0\left(\frac{a^4}{8\ell_{\text{SD}}^4} \exp(4\gamma + 1)\right)}} \approx \frac{4\ell_{\text{SD}}^2}{a} e^{-2\gamma - \frac{1}{2}} = r_1^*, \quad (27)$$

$$r_2^\dagger = a \sqrt{\frac{2}{W_0(2e)}} \approx 1.21a < 2a, \quad (28)$$

$$r_{4,0}^\dagger = a \sqrt{\frac{-2}{W_0\left(-\frac{a^4}{8\ell_{\text{SD}}^4} \exp(4\gamma - 1)\right)}} \approx \frac{4\ell_{\text{SD}}^2}{a} e^{-2\gamma + \frac{1}{2}} = r_4^*, \quad (29)$$

$$r_{4,-1}^\dagger = a \sqrt{\frac{-2}{W_{-1}\left(-\frac{a^4}{8\ell_{\text{SD}}^4} \exp(4\gamma - 1)\right)}} \leq \sqrt{2}a, \quad (30)$$

while  $\lambda_3$  does not have any positive roots. Also note that  $\lambda_4$  has two positive roots,  $r_{4,0}^\dagger$  and  $r_{4,-1}^\dagger$ , corresponding to the principal and lower branches of the Lambert- $W$  function. The roots  $r_2^\dagger$  and  $r_{4,-1}^\dagger$  appear for overlapping particles, while  $r_1^\dagger$  and  $r_{4,0}^\dagger$  are associated with the assumption  $r_{ij} \ll \ell_{\text{SD}}$ . In Fig. 1, we show the roots associated with overlapping particles for both the Stokeslet and Rotne–Prager–Yamakawa-type approximations. We can conclude that the procedure by Rotne and Prager applied to membrane proteins may also lead to the loss of positive definiteness of the mobility tensor if particles overlap, as was also noted in Ref. [7].

## 1.2 Free-standing lipid membranes — general $r_{ij}$

The aggregates considered in this article can reach or exceed the Saffman–Delbrück length scale,  $\ell_{\text{SD}} = \mathcal{O}(1\mu\text{m})$ , such that the assumption  $r_{ij} \ll \ell_{\text{SD}}$ , used in the previous section, may become invalid. Therefore, we now extend the Rotne–Prager–Yamakawa-type tensor to arbitrary interparticle distances. However, carrying out the integral in Eq. (9) for the general case is challenging.

Therefore, we instead employ the multipole expansion approach proposed by Yamakawa [6] since it is conceptually and analytically simpler.

We start by considering the linear force-velocity relation  $\mathbf{v}(\mathbf{x}_i) = \mathbf{G}(\mathbf{x}_i - \mathbf{x}_j)\mathbf{f}(\mathbf{x}_j)$  for the Stokeslet approximation, relating the velocity perturbation at  $\mathbf{x}_i$  to the force acting on particle  $j$  at location  $\mathbf{x}_j$  through the Oseen-type tensor  $\mathbf{G}(\mathbf{x}_i - \mathbf{x}_j)$ . Similarly to before, we define  $\mathbf{r}_{ij} = \mathbf{x}_i - \mathbf{x}_j$  and express  $\mathbf{G}$  as [10]

$$\mathbf{G}(\mathbf{r}_{ij}) = \frac{1}{4\zeta} \left[ \left( H_0\left(\frac{r_{ij}}{\ell_{\text{SD}}}\right) - \frac{\ell_{\text{SD}}}{r_{ij}} H_1\left(\frac{r_{ij}}{\ell_{\text{SD}}}\right) - \frac{1}{2} \left( Y_0\left(\frac{r_{ij}}{\ell_{\text{SD}}}\right) - Y_2\left(\frac{r_{ij}}{\ell_{\text{SD}}}\right) \right) + \frac{2\ell_{\text{SD}}^2}{\pi r_{ij}^2} \right) \mathbf{I}_s \right. \\ \left. - \left( H_0\left(\frac{r_{ij}}{\ell_{\text{SD}}}\right) - \frac{2\ell_{\text{SD}}}{r_{ij}} H_1\left(\frac{r_{ij}}{\ell_{\text{SD}}}\right) + Y_2\left(\frac{r_{ij}}{\ell_{\text{SD}}}\right) + \frac{4\ell_{\text{SD}}^2}{\pi r_{ij}^2} \right) \frac{\mathbf{r}_{ij} \otimes \mathbf{r}_{ij}}{r_{ij}^2} \right], \quad (31)$$

where  $H_k$  and  $Y_k$  are Struve functions and Bessel functions of the second kind, respectively.

Yamakawa proposed to distribute the point force  $\mathbf{f}(\mathbf{x}_i)$  from the Stokeslet approximation over the particle surface and averaging appropriately [6]. For the velocity perturbation due to the force on particle  $j$ , this yields

$$\mathbf{G}^a = \langle \mathbf{G}(\mathbf{r}_{ij} - \mathbf{a}_j) \rangle, \quad (32)$$

where  $\mathbf{a}_j = a\mathbf{e}_r^j$  with  $\mathbf{e}_r^j$  denoting the radial unit vector and the average is taken over the particle circumference. Expanding this expression leads to

$$\mathbf{G}^a \approx \mathbf{G}(\mathbf{r}_{ij}) - \langle \mathbf{a}_j \rangle \cdot \nabla \mathbf{G}|_{\mathbf{r}_{ij}} + \frac{1}{2} \langle \mathbf{a}_j \otimes \mathbf{a}_j \rangle \nabla \nabla \mathbf{G}|_{\mathbf{r}_{ij}} \quad (33)$$

$$= \mathbf{G}(\mathbf{r}_{ij}) + \frac{a^2}{4} \nabla^2 \mathbf{G}|_{\mathbf{r}_{ij}}. \quad (34)$$

Similarly, if we evaluate the velocity at a second finite-size particle  $i \neq j$ , rather than at a point on the membrane, we obtain  $\mathbf{T}_{ij}$  by also averaging over the surface of particle  $i$ , to obtain the tensor

$$\mathbf{T}_{ij} = \langle \mathbf{G}(\mathbf{r}_{ij} - \mathbf{a}_j + \mathbf{a}_i) \rangle, \quad (35)$$

which describes the hydrodynamic interactions between two particles. By expanding around  $\mathbf{r}_{ij}$ , we find

$$\mathbf{T}_{ij} \approx \mathbf{G}(\mathbf{r}_{ij}) - \langle \mathbf{a}_j - \mathbf{a}_i \rangle \cdot \nabla \mathbf{G}|_{\mathbf{r}_{ij}} + \frac{1}{2} \langle (\mathbf{a}_j - \mathbf{a}_i) \otimes (\mathbf{a}_j - \mathbf{a}_i) \rangle : \nabla \nabla \mathbf{G}|_{\mathbf{r}_{ij}} \quad (36)$$

$$= \mathbf{G}(\mathbf{r}_{ij}) + \frac{a^2}{2} \nabla^2 \mathbf{G}|_{\mathbf{r}_{ij}}, \quad (37)$$

where the colon indicates tensor contraction.

To evaluate Eq. (37) for the Saffman–Delbrück case, we first note that the Laplacian of the Oseen tensor can be expressed in the Cartesian basis as

$$\nabla^2 \mathbf{G} = G_{\alpha\beta,\gamma\gamma} \mathbf{e}_\alpha \otimes \mathbf{e}_\beta, \quad (38)$$

where  $G_{\alpha\beta}$  are the components of  $\mathbf{G}$  and the comma denotes the partial derivative, yielding

$$\nabla^2 \mathbf{G}|_{\mathbf{r}_{ij}} = \frac{1}{4\zeta\ell_{\text{SD}}^2} \left[ \left( \frac{2\ell_{\text{SD}}}{\pi r_{ij}} + \frac{1}{2} \left( Y_0\left(\frac{r_{ij}}{\ell_{\text{SD}}}\right) - Y_2\left(\frac{r_{ij}}{\ell_{\text{SD}}}\right) \right) - \left( \frac{\ell_{\text{SD}} H_{-1}\left(\frac{r_{ij}}{\ell_{\text{SD}}}\right)}{r_{ij}} + H_0\left(\frac{r_{ij}}{\ell_{\text{SD}}}\right) \right) \right) \mathbf{I}_s \right. \\ \left. \left( -\frac{2\ell_{\text{SD}}}{\pi r_{ij}} + Y_2\left(\frac{r_{ij}}{\ell_{\text{SD}}}\right) + \frac{2\ell_{\text{SD}} H_{-1}\left(\frac{r_{ij}}{\ell_{\text{SD}}}\right)}{r_{ij}} + H_0\left(\frac{r_{ij}}{\ell_{\text{SD}}}\right) \right) \frac{\mathbf{r}_{ij} \otimes \mathbf{r}_{ij}}{r_{ij}^2} \right]. \quad (39)$$

By inserting this result into Eq. (37), we find

$$\mathbf{T}_{ij}^{\text{SD}}(\mathbf{r}_{ij}) = \frac{1}{4\zeta} \left[ \left( H_0\left(\frac{r_{ij}}{\ell_{\text{SD}}}\right) \left( 1 - \frac{a^2}{2\ell_{\text{SD}}^2} \right) - \frac{a^2}{2\ell_{\text{SD}} r_{ij}} H_{-1}\left(\frac{r_{ij}}{\ell_{\text{SD}}}\right) \right. \right. \\ \left. \left. - \frac{\ell_{\text{SD}}}{r_{ij}} H_1\left(\frac{r_{ij}}{\ell_{\text{SD}}}\right) - \frac{1 - \frac{a^2}{2\ell_{\text{SD}}^2}}{2} \left( Y_0\left(\frac{r_{ij}}{\ell_{\text{SD}}}\right) - Y_2\left(\frac{r_{ij}}{\ell_{\text{SD}}}\right) \right) + \frac{2\ell_{\text{SD}}}{\pi r_{ij}} \left( \frac{\ell_{\text{SD}}}{r_{ij}} + \frac{a^2}{2\ell_{\text{SD}}^2} \right) \right) \mathbf{I}_s \right. \\ \left. - \left( H_0\left(\frac{r_{ij}}{\ell_{\text{SD}}}\right) \left( 1 - \frac{a^2}{2\ell_{\text{SD}}^2} \right) - \frac{a^2 H_{-1}\left(\frac{r_{ij}}{\ell_{\text{SD}}}\right)}{r_{ij} \ell_{\text{SD}}} - \frac{2\ell_{\text{SD}}}{r_{ij}} H_1\left(\frac{r_{ij}}{\ell_{\text{SD}}}\right) + Y_2\left(\frac{r_{ij}}{\ell_{\text{SD}}}\right) \left( 1 - \frac{a^2}{2\ell_{\text{SD}}^2} \right) \right. \right. \\ \left. \left. + \frac{\ell_{\text{SD}}}{\pi r_{ij}} \left( \frac{4\ell_{\text{SD}}}{r_{ij}} + \frac{a^2}{\ell_{\text{SD}}^2} \right) \right) \frac{\mathbf{r}_{ij} \otimes \mathbf{r}_{ij}}{r_{ij}^2} \right]. \quad (40)$$

where we defined  $\alpha = \frac{a^2}{2\ell_{\text{SD}}^2}$ . Expanding around  $r_{ij} = 0$  yields

$$\mathbf{T}_{ij}^{\text{SD}}(\mathbf{r}_{ij}) \approx \frac{1}{4\pi\zeta} \left[ \left( \ln\left(\frac{2\ell_{\text{SD}}}{r_{ij}}\right) - \gamma - \frac{1}{2} + \frac{a^2}{r_{ij}^2} \right) \mathbf{I}_s + \left( 1 - \frac{a^2}{2\ell_{\text{SD}}^2} + \frac{a^2}{\ell_{\text{SD}} r_{ij}} - \frac{2a^2}{r_{ij}^2} \right) \frac{\mathbf{r}_{ij} \otimes \mathbf{r}_{ij}}{r_{ij}^2} \right], \quad (41)$$

and by additionally assuming  $a \ll \ell_{\text{SD}}$ , we recover Eq. (12).

Next, we find the roots of the eigenvalues of  $\mathbf{T}_{ij}^{\text{SD}}$  to ensure that the finite-size mobility tensor does not lose its positive definiteness at large particle distances, as is observed in the Stokeslet approximation. To this end, we identify (cf. Eqs. (14) and (15))

$$f(r_{ij}) = \frac{1}{4\zeta} \left( H_0\left(\frac{r_{ij}}{\ell_{\text{SD}}}\right) \left( 1 - \frac{a^2}{2\ell_{\text{SD}}^2} \right) - \frac{a^2}{2\ell_{\text{SD}} r_{ij}} H_{-1}\left(\frac{r_{ij}}{\ell_{\text{SD}}}\right) - \frac{\ell_{\text{SD}}}{r_{ij}} H_1\left(\frac{r_{ij}}{\ell_{\text{SD}}}\right) \right. \\ \left. - \frac{1}{2} \left( 1 - \frac{a^2}{2\ell_{\text{SD}}^2} \right) \left( Y_0\left(\frac{r_{ij}}{\ell_{\text{SD}}}\right) - Y_2\left(\frac{r_{ij}}{\ell_{\text{SD}}}\right) \right) + \frac{2\ell_{\text{SD}}}{\pi r_{ij}} \left( \frac{\ell_{\text{SD}}}{r_{ij}} + \frac{a^2}{2\ell_{\text{SD}}^2} \right) \right), \quad (42)$$

$$g(r_{ij}) = - \left( H_0\left(\frac{r_{ij}}{\ell_{\text{SD}}}\right) \left( 1 - \frac{a^2}{2\ell_{\text{SD}}^2} \right) - \frac{a^2 H_{-1}\left(\frac{r_{ij}}{\ell_{\text{SD}}}\right)}{r_{ij} \ell_{\text{SD}}} - \frac{2\ell_{\text{SD}}}{r_{ij}} H_1\left(\frac{r_{ij}}{\ell_{\text{SD}}}\right) + Y_2\left(\frac{r_{ij}}{\ell_{\text{SD}}}\right) \left( 1 - \frac{a^2}{2\ell_{\text{SD}}^2} \right) \right. \\ \left. + \frac{\ell_{\text{SD}}}{\pi r_{ij}} \left( \frac{4\ell_{\text{SD}}}{r_{ij}} + \frac{a^2}{\ell_{\text{SD}}^2} \right) \right), \quad (43)$$

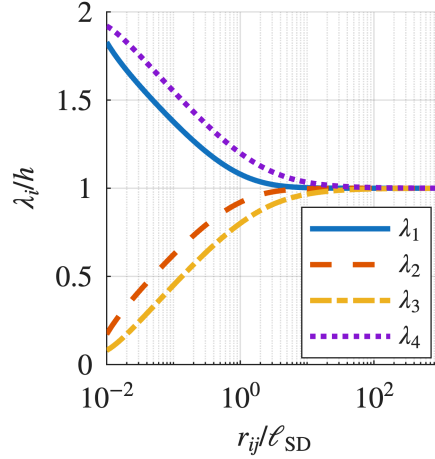

Figure 2: Eigenvalues of  $\mathbf{T}_{ij}^{\text{SD}}$  with finite-size correction for  $a/\ell_{\text{SD}} = 0.005$  and  $r_{ij} > 2a$ . Since  $f$  and  $g$  are decaying with increasing  $r_{ij}$ , we find that the eigenvalues converge to  $h$  at large particle distances.

while  $h$  remains to be given by Eq. (16). The eigenvalues can then be found using Eqs. (19)–(22). For small particle distances, we recover the results discussed in Sec. 1.1. For large particle distances, the resulting expressions are rather intractable. Therefore, we restrict ourselves to plotting the eigenvalues in Fig. (2), revealing that there are no additional roots at large particle distance, implying that the mobility tensor does not lose its positive definiteness.

## 2 Mobility tensor in the Evans–Sackmann theory

In this section, we derive the finite-size mobility tensor for lipid membranes close to a wall using Yamakawa’s method described in Sec. 1.2. We first consider the Stokeslet approximation and subsequently extend the result to account for the finite particle size. Finally, we show that the Rotne–Prager–Yamakawa-type tensor is positive definite for non-overlapping particles.

### 2.1 Stokeslet approximation

We consider a lipid membrane a distance  $h \ll \ell_{\text{SD}}$  away from a rigid wall or substrate (see Fig. (1), main text). In this case, the membrane equations are given by [8, 9, 11]

$$0 = v_{\alpha,\alpha} , \quad (44)$$

$$0 = \lambda_{,\alpha} + \zeta (v_{\beta,\alpha\beta} + v_{\alpha,\beta\beta}) + (\mathbf{t}^+ + \mathbf{t}^-) \cdot \mathbf{e}_\alpha + \mathbf{f} \cdot \mathbf{e}_\alpha \delta(\mathbf{x} - \mathbf{X}) , \quad (45)$$

$$0 = (\mathbf{t}^+ + \mathbf{t}^-) \cdot \mathbf{e}_z , \quad (46)$$

where we use Einstein’s summation convention and Greek indices take values  $\{x, y\}$ . Furthermore,  $\lambda$  denotes the membrane tension,  $v_\alpha$  is the in-plane membrane velocity,  $\mathbf{t}^\pm$  are the tractions acting on the membrane from the bulk domain and  $\mathbf{f}$  is a point force located at  $\mathbf{X}$ . Similarly, the bulk fluid is governed by

$$0 = \text{div} \mathbf{u}^\pm , \quad (47)$$

$$\mathbf{0} = -\nabla p^\pm + \eta \nabla^2 \mathbf{u}_B^\pm , \quad (48)$$



with  $\pm$  referring to the domain above and below the membrane,  $u_{\mathcal{B}}^{\pm}$  and  $p^{\pm}$  denoting the bulk fluid velocity and pressure, respectively, and  $\eta$  being the bulk shear viscosity.

From the above equations, we obtain the Oseen-type tensor in Fourier space as

$$\mathbf{G}(\mathbf{q}) = \frac{1}{\eta q (2\ell_{\text{SD}} q + (1 + \coth hq))} \left( \mathbf{I}_s - \frac{\mathbf{q} \otimes \mathbf{q}}{q^2} \right) e^{-i\mathbf{q} \cdot (\mathbf{x} - \mathbf{X})}, \quad (49)$$

in terms of the two-dimensional wave vector  $\mathbf{q}$ . From  $\coth x \gg 1$  for  $x \ll 1$  and  $1/h \gg 1/\ell_{\text{SD}}$ , it follows that bulk dissipation is dominated by the fluid between the membrane and substrate, implying that the infinite fluid on the other side of the membrane can be neglected [12]. Furthermore, the bulk dissipation on the substrate side only dominates over the membrane dissipation for  $hq \ll 1$  and is negligible otherwise. Therefore, we may expand the hyperbolic cotangent around 0, simplifying Eq. (49) to

$$\mathbf{G}(\mathbf{q}) = \frac{1}{\zeta \left( q^2 + \frac{1}{\ell_{\text{ES}}^2} \right)} \left( \mathbf{I}_s - \frac{\mathbf{q} \otimes \mathbf{q}}{q^2} \right) e^{-i\mathbf{q} \cdot (\mathbf{x} - \mathbf{X})}, \quad (50)$$

where we have now defined the Evans–Sackmann length scale

$$\ell_{\text{ES}} = \sqrt{\frac{h\zeta}{\eta}}. \quad (51)$$

This length scale can be equivalently expressed in terms of an effective friction coefficient  $b \equiv \eta/h$ ,

$$\ell_{\text{ES}} = \sqrt{\frac{\zeta}{b}}. \quad (52)$$

Using this definition, Eq. (50) could be similarly obtained by modeling the contact between the membrane and substrate using the traction  $\mathbf{t}^- = b\mathbf{v}$  as in Ref. [12].

Next, we seek to transform Eq. (50) to physical space, that is

$$\mathbf{G}(\mathbf{x}) = \frac{1}{(2\pi)^2} \int_0^\infty \int_0^{2\pi} \mathbf{G}(\mathbf{q}) q \, d\theta \, dq, \quad (53)$$

expressed in terms of cylindrical coordinates in  $\mathbf{q}$ -space. To simplify the derivation, we express all quantities in terms of a local coordinate system  $\{\mathbf{e}'_x, \mathbf{e}'_y\}$  such that  $\mathbf{r} := \mathbf{x} - \mathbf{X} \propto \mathbf{e}'_y$ . Evaluating the integral along  $\theta$  yields

$$\mathbf{G}(\mathbf{r}) = \frac{1}{4\pi\zeta} \int_0^\infty \frac{1}{q^2 + \frac{1}{\ell_{\text{ES}}^2}} \left( (J_0(qr) - J_2(qr)) \mathbf{I}_s + 2J_2(qr) \frac{\mathbf{r} \otimes \mathbf{r}}{r^2} \right) q \, dq, \quad (54)$$

where  $r = \|\mathbf{x} - \mathbf{X}\|$ . Carrying out the remaining integrals leads to

$$\int_0^\infty \frac{q J_0(qr)}{q^2 + \frac{1}{\ell_{\text{ES}}^2}} \, dq = K_0 \left( \frac{r}{\ell_{\text{ES}}} \right), \quad (55)$$

$$\int_0^\infty \frac{q J_2(qr)}{q^2 + \frac{1}{\ell_{\text{ES}}^2}} \, dq = \frac{2\ell_{\text{ES}}^2}{r^2} - K_2 \left( \frac{r}{\ell_{\text{ES}}} \right), \quad (56)$$

such that we obtain the Oseen tensor in physical space as

$$\mathbf{G}(\mathbf{r}) = \frac{1}{4\pi\zeta} \left( \left( K_0\left(\frac{r}{\ell_{\text{ES}}}\right) + K_2\left(\frac{r}{\ell_{\text{ES}}}\right) - \frac{2\ell_{\text{ES}}^2}{r^2} \right) \mathbf{I}_s + 2 \left( \frac{2\ell_{\text{ES}}^2}{r^2} - K_2\left(\frac{r}{\ell_{\text{ES}}}\right) \right) \frac{\mathbf{r} \otimes \mathbf{r}}{r^2} \right). \quad (57)$$

By further using standard Bessel function recurrence relations, this result can also be written as

$$\begin{aligned} \mathbf{G}(\mathbf{r}) = \frac{1}{2\pi\zeta} & \left( \left( K_0\left(\frac{r}{\ell_{\text{ES}}}\right) + \frac{\ell_{\text{ES}}}{r} K_1\left(\frac{r}{\ell_{\text{ES}}}\right) - \frac{\ell_{\text{ES}}^2}{r^2} \right) \mathbf{I}_s \right. \\ & \left. + \left( \frac{2\ell_{\text{ES}}^2}{r^2} - K_0\left(\frac{r}{\ell_{\text{ES}}}\right) - \frac{2\ell_{\text{ES}}}{r} K_1\left(\frac{r}{\ell_{\text{ES}}}\right) \right) \frac{\mathbf{r} \otimes \mathbf{r}}{r^2} \right). \end{aligned} \quad (58)$$

Equation (58) represents the Oseen tensor for a membrane near a wall and was similarly derived in Ref. [13]. In Sec. 2.3, we show that this result can also be obtained from the original derivation of Evans and Sackmann.

## 2.2 Yamakawa's method for a membrane near a wall

We now apply Yamakawa's method to the Evans–Sackmann case to obtain the corresponding finite-size correction to the Oseen tensor and the Rotne–Prager–Yamakawa-type mobility tensor using Eqs. (34) and (37), respectively. Evaluating the Laplacian of Eq. (58) yields

$$\nabla^2 \mathbf{G}(\mathbf{r}) = \frac{1}{2\pi\zeta\ell_{\text{ES}}^2} \left( \left( K_0\left(\frac{r}{\ell_{\text{ES}}}\right) + \frac{\ell_{\text{ES}}}{r} K_1\left(\frac{r}{\ell_{\text{ES}}}\right) \right) \mathbf{I}_s - \left( K_0\left(\frac{r}{\ell_{\text{ES}}}\right) + \frac{2\ell_{\text{ES}}}{r} K_1\left(\frac{r}{\ell_{\text{ES}}}\right) \right) \frac{\mathbf{r} \otimes \mathbf{r}}{r^2} \right), \quad (59)$$

leading to

$$\begin{aligned} \mathbf{G}^a = \frac{1}{2\pi\zeta} & \left\{ \left[ \left( K_0\left(\frac{r}{\ell_{\text{ES}}}\right) + \frac{\ell_{\text{ES}}}{r} K_1\left(\frac{r}{\ell_{\text{ES}}}\right) \right) \left( 1 + \frac{a^2}{4\ell_{\text{ES}}^2} \right) - \frac{\ell_{\text{ES}}^2}{r^2} \right] \mathbf{I}_s \right. \\ & \left. + \left[ \frac{2\ell_{\text{ES}}^2}{r^2} - \left( K_0\left(\frac{r}{\ell_{\text{ES}}}\right) + \frac{2\ell_{\text{ES}}}{r} K_1\left(\frac{r}{\ell_{\text{ES}}}\right) \right) \left( 1 + \frac{a^2}{4\ell_{\text{ES}}^2} \right) \right] \frac{\mathbf{r} \otimes \mathbf{r}}{r^2} \right\}. \end{aligned} \quad (60)$$

Equation (60) is the finite-size correction to the Stokeslet approximation in Eq. (58). In Sec. 2.3, we show that this result provides a good approximation to the flow field obtained by Evans and Sackmann in their original derivation. Finally, we use Eq. (37) to obtain the finite-size correction to the mobility tensor as

$$\begin{aligned} \mathbf{T}_{ij}^{\text{ES}} = \frac{1}{2\pi\zeta} & \left\{ \left[ \left( K_0\left(\frac{r_{ij}}{\ell_{\text{ES}}}\right) + \frac{\ell_{\text{ES}}}{r_{ij}} K_1\left(\frac{r_{ij}}{\ell_{\text{ES}}}\right) \right) \left( 1 + \frac{a^2}{2\ell_{\text{ES}}^2} \right) - \frac{\ell_{\text{ES}}^2}{r_{ij}^2} \right] \mathbf{I}_s \right. \\ & \left. + \left[ \frac{2\ell_{\text{ES}}^2}{r_{ij}^2} - \left( K_0\left(\frac{r_{ij}}{\ell_{\text{ES}}}\right) + \frac{2\ell_{\text{ES}}}{r_{ij}} K_1\left(\frac{r_{ij}}{\ell_{\text{ES}}}\right) \right) \left( 1 + \frac{a^2}{2\ell_{\text{ES}}^2} \right) \right] \frac{\mathbf{r}_{ij} \otimes \mathbf{r}_{ij}}{r_{ij}^2} \right\}, \end{aligned} \quad (61)$$

where we have now used the notation  $\mathbf{r} \rightarrow \mathbf{r}_{ij}$  for consistency.

### 2.3 Stokeslet approximation based on original Evans–Sackmann derivation

We can also obtain the Oseen tensor, including a finite-size correction, directly from the work of Evans and Sackmann [12]. The authors obtain the velocity profile due to a force  $\mathbf{F}$  acting on a cylindrical inclusion with radius  $a$  at point  $\mathbf{x}$  as

$$\mathbf{v}(\mathbf{x}') = (\tilde{v}_r(r) \cos \phi \mathbf{e}_r + \tilde{v}_\phi(r) \sin \phi \mathbf{e}_\phi) \mathbf{F} , \quad (62)$$

where  $r$  and  $\phi$  are the radial and azimuthal coordinates at  $\mathbf{x}' = \mathbf{x} + r\mathbf{e}_r(\phi)$ , respectively,  $\mathbf{e}_r$  and  $\mathbf{e}_\phi$  are the corresponding basis vectors,  $\mathbf{F} = F\mathbf{e}_r|_{\phi=0}$ , and  $\tilde{v}_r$  and  $\tilde{v}_\phi$  are given by [12]

$$\tilde{v}_r = \frac{1}{\pi\zeta \left(1 + \frac{4K_1(\varepsilon)}{\varepsilon K_0(\varepsilon)}\right)} \left( \frac{\ell_{\text{ES}}^2}{r^2} \left(1 + \frac{2K_1(\varepsilon)}{\varepsilon K_0(\varepsilon)}\right) - \frac{2\ell_{\text{ES}}}{r\varepsilon^2 K_0(\varepsilon)} K_1\left(\frac{r}{\ell_{\text{ES}}}\right) \right) , \quad (63)$$

$$\tilde{v}_\phi = \frac{1}{\pi\zeta \left(1 + \frac{4K_1(\varepsilon)}{\varepsilon K_0(\varepsilon)}\right)} \left( \frac{\ell_{\text{ES}}^2}{r^2} \left(1 + \frac{2K_1(\varepsilon)}{\varepsilon K_0(\varepsilon)}\right) - \frac{2\ell_{\text{ES}}}{r\varepsilon^2 K_0(\varepsilon)} \left( \frac{r}{\ell_{\text{ES}}} K_0\left(\frac{r}{\ell_{\text{ES}}}\right) + K_1\left(\frac{r}{\ell_{\text{ES}}}\right) \right) \right) , \quad (64)$$

where  $r = \|\mathbf{x} - \mathbf{x}'\|$ ,  $\zeta$  is the membrane viscosity and  $K_i$  are modified Bessel functions of the second kind. Furthermore, the nondimensional radius is defined as

$$\varepsilon = \frac{a}{\ell_{\text{ES}}} . \quad (65)$$

We can obtain the finite-size correction to the Oseen tensor,  $\mathbf{G}^a$ , from Eqs. (62)–(64). To this end, we note

$$\mathbf{F} \cdot \mathbf{e}_r = F \cos \phi , \quad (66)$$

$$\mathbf{F} \cdot \mathbf{e}_\phi = -F \sin \phi . \quad (67)$$

Thus, we can rewrite Eq. (62) as

$$\mathbf{v}(\mathbf{x}') = (\tilde{v}_r \mathbf{e}_r \otimes \mathbf{e}_r - \tilde{v}_\phi \mathbf{e}_\phi \otimes \mathbf{e}_\phi) \mathbf{F} \quad (68)$$

$$= \left( (\tilde{v}_r + \tilde{v}_\phi) \frac{\mathbf{r} \otimes \mathbf{r}}{r^2} - \tilde{v}_\phi \mathbf{I}_s \right) \mathbf{F} , \quad (69)$$

with  $\mathbf{R} = \mathbf{x}' - \mathbf{x}$  and  $\mathbf{I}_s$  denoting the in-plane identity tensor. From Eq. (69), we immediately infer the finite-size Oseen tensor as

$$\mathbf{G}^a(\mathbf{r}) = -\tilde{v}_\phi \mathbf{I}_s + (\tilde{v}_r + \tilde{v}_\phi) \frac{\mathbf{r} \otimes \mathbf{r}}{r^2} . \quad (70)$$

In the limit of  $a \rightarrow 0$ , Eqs. (63) and (64) reduce to

$$\lim_{a \rightarrow 0} \tilde{v}_r = \frac{1}{2\pi\zeta} \left( \frac{\ell_{\text{ES}}^2}{r^2} - \frac{\ell_{\text{ES}}}{r} K_1\left(\frac{r}{\ell_{\text{ES}}}\right) \right) , \quad (71)$$

$$\lim_{a \rightarrow 0} \tilde{v}_\phi = \frac{1}{2\pi\zeta} \left( \frac{\ell_{\text{ES}}^2}{r^2} - K_0\left(\frac{r}{\ell_{\text{ES}}}\right) - \frac{\ell_{\text{ES}}}{r} K_1\left(\frac{r}{\ell_{\text{ES}}}\right) \right) . \quad (72)$$

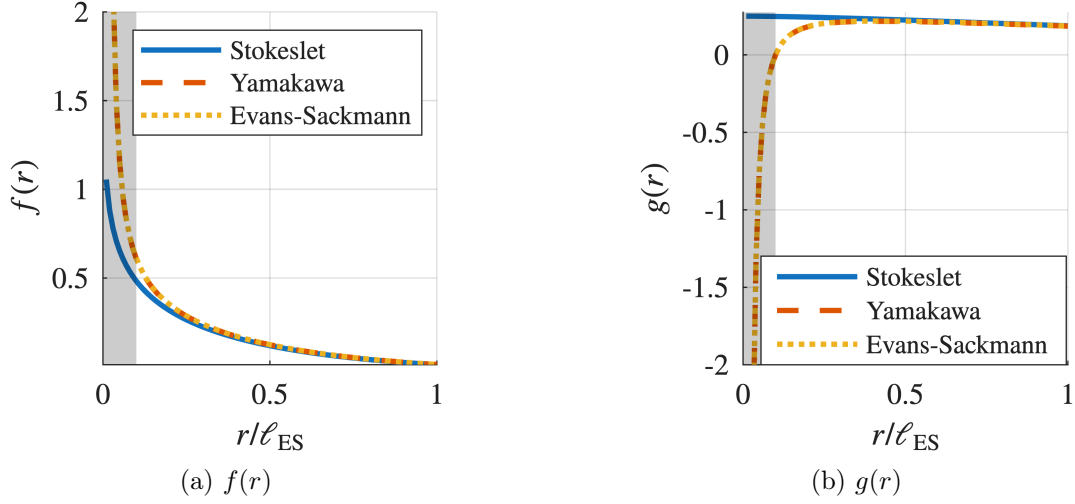

Figure 3: Comparison of the Oseen-type tensors for a membrane near a wall using the Stokeslet approximation (Eq. (58)), Yamakawa’s method (Eq. (60)), and the original result of Evans and Sackmann (Eq. (73) for  $a = 0.1\ell_{\text{ES}}$ ). The gray area indicates the region occupied by the particle. For easier comparison, we express the Oseen-type tensors as  $f(r)\mathbf{I}_s + g(r)\frac{\mathbf{r}\otimes\mathbf{r}}{r^2}$ . The results show that Yamakawa’s method provides an excellent approximation for the original result by Evans and Sackmann.

By substituting these expressions into Eq. (70), we obtain the Oseen tensor in the Stokeslet approximation (cf. Eq. (58) and Ref. [13]). Finally, substituting Eqs. (63) and (64) into Eq. (70) results in the finite-size correction to the Oseen tensor,

$$\mathbf{G}^a = \frac{1}{\pi\zeta\left(1 + \frac{4K_1(\varepsilon)}{\varepsilon K_0(\varepsilon)}\right)} \left[ -\left(\frac{\ell_{\text{ES}}^2}{r^2} \left(1 + \frac{2K_1(\varepsilon)}{\varepsilon K_0(\varepsilon)}\right) - \frac{2\ell_{\text{ES}}}{r\varepsilon^2 K_0(\varepsilon)} \left(\frac{r}{\ell_{\text{ES}}} K_0\left(\frac{r}{\ell_{\text{ES}}}\right) + K_1\left(\frac{r}{\ell_{\text{ES}}}\right)\right)\right) \mathbf{I} \right. \\ \left. + \left(\frac{2\ell_{\text{ES}}^2}{r^2} \left(1 + \frac{2K_1(\varepsilon)}{\varepsilon K_0(\varepsilon)}\right) - \frac{2\ell_{\text{ES}}}{r\varepsilon^2 K_0(\varepsilon)} \left(\frac{r}{\ell_{\text{ES}}} K_0\left(\frac{r}{\ell_{\text{ES}}}\right) + 2K_1\left(\frac{r}{\ell_{\text{ES}}}\right)\right)\right) \frac{\mathbf{r}\otimes\mathbf{r}}{r^2} \right]. \quad (73)$$

In Fig. (3), we compare the Stokeslet approximation (Eq. (58)) and Yamakawa’s method (Eq. (60)) to Eq. (73) by generically expressing the results as  $\mathbf{G}^a = f(r)\mathbf{I}_s + g(r)\frac{\mathbf{r}\otimes\mathbf{r}}{r^2}$ . This shows good agreement between the results from Evans and Sackmann and Yamakawa’s method. In contrast, the Stokeslet approximation only provides a good approximation sufficiently far from the particle.

## 2.4 Positive definiteness of the mobility tensor

In this section, we will investigate the positive definiteness of the mobility tensor resulting from the Stokeslet and Rotne–Prager–Yamakawa approximations. To this end, we again write the mobility tensor using the generic form

$$\mathbf{T}_{ij}^{\text{ES}} = f(r)\mathbf{I}_s + g(r)\frac{\mathbf{r}\otimes\mathbf{r}}{r^2}. \quad (74)$$

Additionally, we define

$$h = \frac{1}{4\pi\zeta} \underbrace{\left[ \left( \frac{a}{2\ell_{\text{ES}}} \right)^2 + \frac{a}{\ell_{\text{ES}}} \frac{K_1\left(\frac{a}{\ell_{\text{ES}}}\right)}{K_0\left(\frac{a}{\ell_{\text{ES}}}\right)} \right]}_{=:2\mu(a)}^{-1}, \quad (75)$$

such that the eigenvalues are given by Eqs. (19)–(22).

We begin by considering the Stokeslet approximation, where the Oseen tensor is given by Eq. (58). Since we expect the loss of positive definiteness to occur for small particle distances, we expand  $f(r)$  and  $g(r)$  around  $r/\ell_{\text{ES}} = 0$ ,

$$f(r) = K_0\left(\frac{r}{\ell_{\text{ES}}}\right) + \frac{\ell_{\text{ES}}}{r} K_1\left(\frac{r}{\ell_{\text{ES}}}\right) - \frac{\ell_{\text{ES}}^2}{r^2} \quad (76)$$

$$\approx -\frac{1}{2} \left( \ln \frac{r}{2\ell_{\text{ES}}} + \gamma + \frac{1}{2} \right), \quad (77)$$

$$g(r) = \frac{2\ell_{\text{ES}}^2}{r^2} - K_0\left(\frac{r}{\ell_{\text{ES}}}\right) - \frac{2\ell_{\text{ES}}}{r} K_1\left(\frac{r}{\ell_{\text{ES}}}\right) \approx \frac{1}{2}. \quad (78)$$

As in Sec. 1.1, we solve for the roots of the eigenvalues, yielding

$$r_1^* = 2\ell_{\text{ES}} \exp\left(2\mu(a) - \gamma - \frac{1}{2}\right), \quad (79)$$

$$r_2^* = 2\ell_{\text{ES}} \exp\left(-\left(2\mu(a) + \gamma + \frac{1}{2}\right)\right), \quad (80)$$

$$r_3^* = 2\ell_{\text{ES}} \exp\left(-2\mu(a) - \gamma + \frac{1}{2}\right), \quad (81)$$

$$r_4^* = 2\ell_{\text{ES}} \exp\left(2\mu(a) - \gamma + \frac{1}{2}\right). \quad (82)$$

The asymptotic behavior of  $\lambda_1$  and  $\lambda_4$  suggests that these roots are artifacts of the expansions in Eqs. (77) and (78) and should not be considered further. In contrast,  $r_2^*$  and  $r_3^*$  are approximations of the true roots of  $\lambda_2$  and  $\lambda_3$ , respectively. Expanding  $\mu(a)$  for  $a \ll \ell_{\text{ES}}$  then yields

$$r_2^* = ae^{-\frac{1}{2}} \approx 0.61a, \quad (83)$$

$$r_3^* \approx ae^{\frac{1}{2}} \approx 1.65a. \quad (84)$$

These results coincide with the Saffman–Delbrück results in Eqs. (24) and (25). Thus, we find that the Stokeslet approximation can lead to the loss of positive definiteness of the mobility tensor for overlapping particles.

Next, we consider the Rotne–Prager–Yamakawa-type tensor in Eq. (61). Similarly to the

Stokeslet approximation, we define  $f(r)$  and  $g(r)$  and expand them around  $r/\ell_{\text{ES}} = 0$ ,

$$f(r) = \left( K_0 \left( \frac{r}{\ell_{\text{ES}}} \right) + \frac{\ell_{\text{ES}}}{r} K_1 \left( \frac{r}{\ell_{\text{ES}}} \right) \right) \left( 1 + \frac{a^2}{2\ell_{\text{ES}}^2} \right) - \frac{\ell_{\text{ES}}^2}{r^2} \quad (85)$$

$$\approx \frac{a^2}{2r^2} - \frac{1}{2} \left( \frac{a^2}{2\ell_{\text{ES}}} + 1 \right) \left( \ln \frac{r}{2\ell_{\text{ES}}} + \gamma + \frac{1}{2} \right), \quad (86)$$

$$g(r) = \frac{2\ell_{\text{ES}}^2}{r^2} - \left( K_0 \left( \frac{r}{\ell_{\text{ES}}} \right) + \frac{2\ell_{\text{ES}}}{r} K_1 \left( \frac{r}{\ell_{\text{ES}}} \right) \right) \left( 1 + \frac{a^2}{2\ell_{\text{ES}}^2} \right) \approx -\frac{a^2}{r^2} + \frac{a^2 + 2\ell_{\text{ES}}^2}{4\ell_{\text{ES}}^2}. \quad (87)$$

Analogously to Sec. 1.1, we now find that  $\lambda_3$  is positive for all values of  $r$  and that the roots of  $\lambda_1$ ,  $\lambda_2$ , and  $\lambda_4$  are given by

$$r_1^\dagger = \frac{2\ell_{\text{ES}}a}{\sqrt{a^2 + 2\ell_{\text{ES}}^2}} \frac{1}{\sqrt{W_0 \left( \frac{a^2}{a^2 + 2\ell_{\text{ES}}^2} \exp \left( 2 \left( \gamma + \frac{1}{2} \right) - \frac{4\mu(a)}{\frac{a^2}{2\ell_{\text{ES}}^2} + 1} \right) \right)}} \quad (88)$$

$$\approx \frac{4\ell_{\text{ES}}^2}{a \exp(2\gamma + \frac{1}{2})} > 2a, \quad (89)$$

$$r_2^\dagger = \frac{2\ell_{\text{ES}}a}{\sqrt{a^2 + 2\ell_{\text{ES}}^2}} \frac{1}{\sqrt{W_0 \left( \frac{a^2}{a^2 + 2\ell_{\text{ES}}^2} \exp \left( 2 \left( \gamma + \frac{1}{2} \right) + \frac{4\mu(a)}{\frac{a^2}{2\ell_{\text{ES}}^2} + 1} \right) \right)}} \quad (90)$$

$$\approx \frac{\sqrt{2}a}{\sqrt{\ln 2 + 1}} < 2a, \quad (91)$$

$$r_{4,0}^\dagger = \frac{2i\ell_{\text{ES}}a}{\sqrt{a^2 + 2\ell_{\text{ES}}^2}} \frac{1}{\sqrt{W_0 \left( -\frac{a^2}{a^2 + 2\ell_{\text{ES}}^2} \exp \left( 2 \left( \gamma + \frac{1}{2} \right) - 2 \left( 1 + \frac{4\ell_{\text{ES}}^2\mu(a)}{a^2 + 2\ell_{\text{ES}}^2} \right) \right) \right)}} \quad (92)$$

$$\approx 2\ell_{\text{ES}} \exp \left( \frac{1}{2} - \frac{2\ell_{\text{ES}}^2 (\ln \frac{a}{2} + \gamma)}{a^2 + 2\ell_{\text{ES}}^2} - \gamma \right), \quad (93)$$

$$r_{4,-1}^\dagger = \frac{2i\ell_{\text{ES}}a}{\sqrt{a^2 + 2\ell_{\text{ES}}^2}} \frac{1}{\sqrt{W_{-1} \left( -\frac{a^2}{a^2 + 2\ell_{\text{ES}}^2} \exp \left( 2 \left( \gamma + \frac{1}{2} \right) - 2 \left( 1 + \frac{4\ell_{\text{ES}}^2\mu(a)}{a^2 + 2\ell_{\text{ES}}^2} \right) \right) \right)}} \quad (94)$$

$$\leq 2a \frac{\ell_{\text{ES}}}{\sqrt{a^2 + 2\ell_{\text{ES}}^2}} < 2a. \quad (95)$$

Here, the approximations in Eqs. (89), (91), and (93) assume  $a/\ell_{\text{ES}} \ll 1$ . The roots  $r_1^\dagger$  and  $r_{4,-1}^\dagger$  are artifacts of the expansion around small  $r$  and are therefore not physically relevant. In contrast,  $r_2^\dagger$  and  $r_{4,0}^\dagger$  indeed indicate a loss of positive definiteness for small particle distances. However, as for the Saffman–Delbrück case and in the Stokeslet approximation for the Evans–Sackmann case, this occurs only for overlapping particles, as shown in Fig. 4a. Finally, to confirm that all eigenvalues remain positive at large distances, they are plotted in Fig. 4b for a fixed particle size.

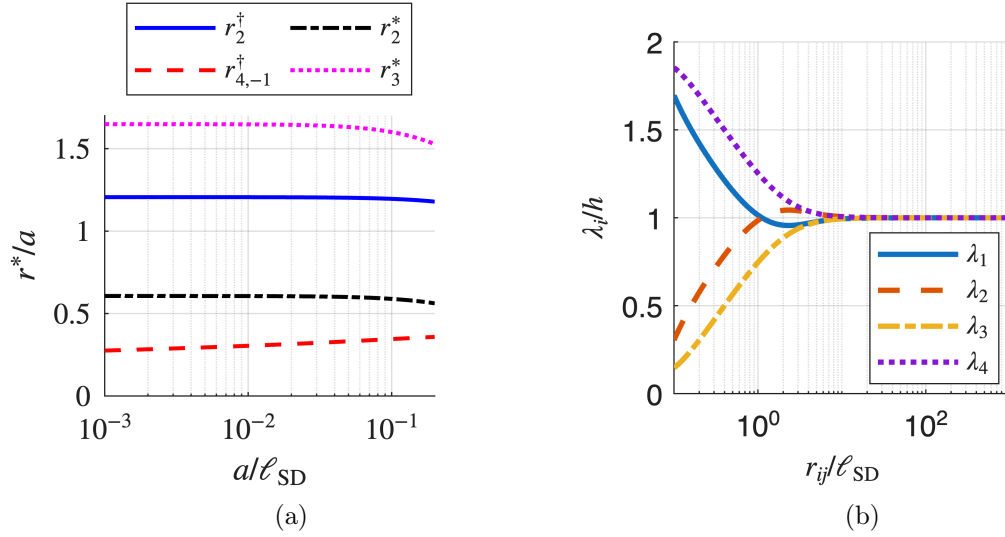

Figure 4: Roots of eigenvalues for the Stokeslet (\*) and Rotne-Prager-Yamakawa-type approximations (†) for small particle distances in (a) and eigenvalues of the Rotne-Prager-Yamakawa-type tensor for  $a/\ell_{\text{SD}} = 0.05$  and  $r > 2a$  in (b).

### 3 Derivation of the hydrodynamic radii

To derive the hydrodynamic radii for different membrane protein aggregates, we follow the approach proposed by Bloomfield et al. [14]. We first recall the self-consistent force balance provided by Kirkwood-Riseman theory,

$$\mathbf{F}_i = -\xi (\mathbf{v}_i^0 - \mathbf{u}_i) - \xi \sum_{\substack{j=1 \\ j \neq i}}^N \mathbf{T}_{ij} \mathbf{F}_j . \quad (96)$$

Summing over all forces then yields

$$\mathbf{F} = \sum_i \mathbf{F}_i = -\sum_i \xi (\mathbf{v}_i^0 - \mathbf{u}_i) - \xi \sum_{i=1}^N \sum_{\substack{j=1 \\ j \neq i}}^N \mathbf{T}_{ij} \mathbf{F}_j . \quad (97)$$

For  $\mathbf{w} = (\mathbf{v}_i^0 - \mathbf{u}_i)$  independent of  $i$ , this can be rewritten as

$$\mathbf{F} = -N\xi \left( \mathbf{w} + \frac{1}{N} \sum_{i=1}^N \sum_{\substack{j=1 \\ j \neq i}}^N \mathbf{T}_{ij} \mathbf{F}_j \right) . \quad (98)$$

Bloomfield et al. [14] then make the ansatz that Eq. (96) can be approximated as

$$\mathbf{F}_j \approx -\xi \mathbf{w} . \quad (99)$$

Substituting Eq. (99) into Eq. (98) leads to

$$\mathbf{F} = -N\xi \left( \mathbf{I}_s - \frac{\xi}{N} \sum_{i=1}^N \sum_{\substack{j=1 \\ j \neq i}}^N \mathbf{T}_{ij} \right) \mathbf{w} . \quad (100)$$

This motivates the definition of the friction coefficient tensor as

$$\Xi = N\xi \left( \mathbf{I}_s - \frac{\xi}{N} \sum_{i=1}^N \sum_{\substack{j=1 \\ j \neq i}}^N \mathbf{T}_{ij} \right) , \quad (101)$$

which can be *approximately* inverted to give [14, 15]

$$\Xi^{-1} \approx \frac{1}{N\xi} \left( \mathbf{I}_s + \frac{\xi}{N} \sum_{i=1}^N \sum_{\substack{j=1 \\ j \neq i}}^N \mathbf{T}_{ij} \right) \quad (102)$$

Following Ref. [14], the scalar drag coefficient is then defined by

$$\frac{1}{\Xi} = \frac{1}{2} \text{tr} \Xi^{-1} \quad (103)$$

$$= \frac{1}{N\xi} + \frac{1}{2N^2} \sum_{i=1}^N \sum_{\substack{j=1 \\ j \neq i}}^N \text{tr} \mathbf{T}_{ij} \quad (104)$$

which is related to the aggregate diffusion coefficient  $D_N$  by the Einstein relation,

$$D_N = \frac{k_B T}{\Xi} , \quad (105)$$

in terms of the Boltzmann constant  $k_B$  and temperature  $T$ .

Equations (104) and (105) now lead to the definition of the hydrodynamic radius  $R_H$ . Given an expression for the diffusivity of a single particle with radius  $a$ , say  $D_1 = \mathcal{D}(a)$ , we *define* the hydrodynamic radius by the relation

$$\mathcal{D}(R_H) = \frac{k_B T}{\Xi} , \quad (106)$$

such that the diffusion coefficient of the aggregate satisfies the same relation as the diffusion coefficient of a single particle. In the following two sections, we apply this approach to derive the hydrodynamic radii for the Saffman–Delbrück and Evans–Sackmann cases.

### 3.1 Free-standing membrane

To evaluate the hydrodynamic radius of a protein aggregate on a free-standing membrane, we evaluate the trace of the Rotne–Prager–Yamakawa-type tensor in Eq. (40), yielding

$$\text{tr}(\mathbf{T}_{ij}^{\text{SD}}) = \frac{1}{4\zeta} \left( \frac{a^2}{\pi r_{ij} \ell_{\text{SD}}} + \left( 1 - \frac{a^2}{2\ell_{\text{SD}}^2} \right) \left( H_0 \left( \frac{r_{ij}}{\ell_{\text{SD}}} \right) - Y_0 \left( \frac{r_{ij}}{\ell_{\text{SD}}} \right) \right) \right) . \quad (107)$$



In contrast to the three-dimensional case [15], Eq. (107) suggests that the particle radius enters the hydrodynamic radius. However, from  $a \ll \ell_{\text{SD}}$ , we can reduce Eq. (107) to

$$\text{tr}(\mathbf{T}_{ij}^{\text{SD}}) \approx \frac{1}{4\zeta} \left( H_0 \left( \frac{r_{ij}}{\ell_{\text{SD}}} \right) - Y_0 \left( \frac{r_{ij}}{\ell_{\text{SD}}} \right) \right), \quad (108)$$

independent of the particle radius  $a$ . Inserting this result into Eq. (106) with

$$\mathcal{D}(R_{\text{H}}^{\text{SD}}) = \frac{k_{\text{B}}T}{4\pi\zeta} \left( \ln \frac{2\ell_{\text{SD}}}{R_{\text{H}}^{\text{SD}}} - \gamma \right), \quad (109)$$

we find the hydrodynamic radius as

$$R_{\text{H}}^{\text{SD}} = 2\ell_{\text{SD}} \left( \frac{a}{2\ell_{\text{SD}}} \right)^{1/N} \exp \left( -\frac{\pi}{2N^2} \sum_{i=1}^N \sum_{\substack{j=1 \\ j \neq i}}^N \left( H_0 \left( \frac{r_{ij}}{\ell_{\text{SD}}} \right) - Y_0 \left( \frac{r_{ij}}{\ell_{\text{SD}}} \right) \right) - \frac{\gamma(N-1)}{N} \right). \quad (110)$$

This result is discussed in more detail in the main text.

### 3.2 Membrane near a wall

To obtain the hydrodynamic radius for a protein aggregate on a membrane near a wall, taking the trace of Eq. (61) leads to

$$\text{tr}(\mathbf{T}_{ij}^{\text{ES}}) = \frac{1}{2\pi\zeta} \left( 1 - \frac{a^2}{2\ell_{\text{ES}}^2} \right) K_0 \left( \frac{r_{ij}}{\ell_{\text{ES}}} \right). \quad (111)$$

We note that for large particles and small distances between the membrane and wall, the ratio  $a/\ell_{\text{ES}}$  is not necessarily small. Thus, the dependence on the particle radius may not vanish in the Evans–Sackmann case.

For a membrane near a wall, the left-hand side of Eq. (106) is given by

$$\mathcal{D}(R_{\text{H}}^{\text{ES}}) = \frac{k_{\text{B}}T}{4\pi\zeta} \left( \left( \frac{R_{\text{H}}^{\text{ES}}}{2\ell_{\text{ES}}} \right)^2 + \frac{R_{\text{H}}^{\text{ES}}}{\ell_{\text{ES}}} \frac{K_1 \left( \frac{R_{\text{H}}^{\text{ES}}}{\ell_{\text{ES}}} \right)}{K_0 \left( \frac{R_{\text{H}}^{\text{ES}}}{\ell_{\text{ES}}} \right)} \right)^{-1}. \quad (112)$$

Evidently, Eq. (112) does not yield an analytical expression for the hydrodynamic radius when substituted into Eq. (106). Therefore, we consider the cases of small and large hydrodynamic radii below.

Beginning with the case  $R_{\text{H}}^{\text{ES}} \ll \ell_{\text{ES}}$ , we note that this assumption also suggests  $a \ll \ell_{\text{ES}}$ . Thus, Eq. (111) simplifies to

$$\text{tr}(\mathbf{T}_{ij}^{\text{ES}}) = \frac{1}{2\pi\zeta} K_0 \left( \frac{r_{ij}}{\ell_{\text{ES}}} \right). \quad (113)$$

Furthermore, for  $R_{\text{H}}^{\text{ES}} \ll \ell_{\text{ES}}$ ,  $\mathcal{D}(R_{\text{H}}^{\text{ES}})$  reduces to

$$\mathcal{D}(R_{\text{H}}^{\text{ES},s}) \approx \frac{k_{\text{B}}T}{4\pi\zeta} \left( \ln \left( \frac{2\ell_{\text{ES}}}{R_{\text{H}}^{\text{ES},s}} \right) - \gamma \right), \quad (114)$$

where  $R_H^{\text{ES},s}$  is the hydrodynamic radius of small aggregates. Solving for  $R_H^{\text{ES},s}$  then yields

$$R_H^{\text{ES},s} = 2\ell_{\text{ES}} \left( \frac{a}{2\ell_{\text{ES}}} \right)^{1/N} \exp \left( -\frac{1}{N^2} \sum_{i=1}^N \sum_{\substack{j=1 \\ j \neq i}}^N K_0 \left( \frac{r_{ij}}{\ell_{\text{ES}}} \right) - \frac{\gamma(N-1)}{N} \right), \quad (115)$$

where we have also expanded the single-particle drag coefficients for  $a \ll \ell_{\text{ES}}$ .

When we consider the case of large aggregates, i.e.  $R_H^{\text{ES}} \gg \ell_{\text{ES}}$ , we can express  $\mathcal{D}(R_H^{\text{ES}})$  as

$$\mathcal{D}(R_H^{\text{ES},1}) \approx \frac{k_B T}{\pi \zeta} \frac{\ell_{\text{ES}}^2}{R_H^2}, \quad (116)$$

in terms of the large-aggregate hydrodynamic radius  $R_H^{\text{ES},1}$ . Again solving for the hydrodynamic radius yields

$$R_H^{\text{ES},1} = \frac{2\ell_{\text{ES}} N}{\sqrt{2N\mu(a) + \left(1 - \frac{a^2}{2\ell_{\text{ES}}^2}\right) \sum_{i=1}^N \sum_{j=1, j \neq i}^N K_0 \left( \frac{r_{ij}}{\ell_{\text{ES}}} \right)}} \quad (117)$$

$$= \frac{2\ell_{\text{ES}}}{\sqrt{\frac{4\pi\zeta}{N\xi_{\text{ES}}} + \left(1 - \frac{a^2}{2\ell_{\text{ES}}^2}\right) \frac{1}{N^2} \sum_{i=1}^N \sum_{j=1, j \neq i}^N K_0 \left( \frac{r_{ij}}{\ell_{\text{ES}}} \right)}}, \quad (118)$$

where  $\xi_{\text{ES}}$  is the single-particle drag coefficient.

## References

- [1] Kirkwood, J. G. & Riseman, J. The intrinsic viscosities and diffusion constants of flexible macromolecules in solution. *The Journal of Chemical Physics* **16**, 565–573 (1948).
- [2] Zwanzig, R., Kiefer, J. & Weiss, G. H. On the validity of the Kirkwood-Riseman theory. *Proceedings of the National Academy of Sciences* **60**, 381–386 (1968).
- [3] Zuk, P. J., Wajnryb, E., Mizerski, K. & Szymczak, P. Rotne–Prager–Yamakawa approximation for different-sized particles in application to macromolecular bead models. *Journal of Fluid Mechanics* **741**, R5 (2014).
- [4] DeWames, R., Hall, W. & Shen, M. On the molecular theories of polymer solutions. *The Journal of Chemical Physics* **46**, 2782–2794 (1967).
- [5] Rotne, J. & Prager, S. Variational treatment of hydrodynamic interaction in polymers. *The Journal of Chemical Physics* **50**, 4831–4837 (1969).
- [6] Yamakawa, H. Transport properties of polymer chains in dilute solution: hydrodynamic interaction. *The Journal of Chemical Physics* **53**, 436–443 (1970).
- [7] Sokolov, Y. & Diamant, H. Many-particle mobility and diffusion tensors for objects in viscous sheets. *The Journal of Chemical Physics* **149** (2018).

- [8] Sahu, A., Sauer, R. A. & Mandadapu, K. K. Irreversible thermodynamics of curved lipid membranes. *Physical Review E* **96**, 042409 (2017).
- [9] Omar, Y. A., Lipel, Z. G. & Mandadapu, K. K.  $(2+\delta)$ -dimensional theory of the electromechanics of lipid membranes. III. Constitutive models. *Physical Review E* **112**, 024407 (2025).
- [10] Oppenheimer, N. & Diamant, H. Correlated diffusion of membrane proteins and their effect on membrane viscosity. *Biophysical Journal* **96**, 3041–3049 (2009).
- [11] Goutaland, Q. & Fournier, J.-B. Saffman-Delbrück and beyond: A pointlike approach. *The European Physical Journal E* **42**, 156 (2019).
- [12] Evans, E. & Sackmann, E. Translational and rotational drag coefficients for a disk moving in a liquid membrane associated with a rigid substrate. *Journal of Fluid Mechanics* **194**, 553–561 (1988).
- [13] Ramachandran, S., Komura, S., Seki, K. & Gompper, G. Dynamics of a polymer chain confined in a membrane. *The European Physical Journal E* **34**, 46 (2011).
- [14] Bloomfield, V., Dalton, W. & Van Holde, K. Frictional coefficients of multisubunit structures. I. Theory. *Biopolymers: Original Research on Biomolecules* **5**, 135–148 (1967).
- [15] GarciadelaTorre, J. & Bloomfield, V. Hydrodynamic properties of macromolecular complexes. 1. Translation. *Biopolymers* **16**, 1747–1763 (1977).
